# Supplementary material for: SIXO: Smoothing Inference with Twisted Objectives
Source: arXiv:2206.05952 source file (2022-06-20)
Supplement: Supplementary file 1 [file app_05_related_work.tex]

\section{Related Work}

\subsection{Twisting}
\todo{This all needs careful review to make sure i'm right}  We can therefore use twists to preemptively increase the probability of particles, at time $t$, given information available beyond $t+1$.  \citet{lin2013lookahead} provide an extensive summary of look ahead techniques, and present methods using \emph{pilot particles} to estimate the look-ahead distribution numerically.  These ideas were first introduced by \citet{pitt1999filtering}, with the \emph{auxiliary particle filter} (APF), where an estimate of the one-step backwards message $p_{\btheta}(\by_{t+1} \mid \bx_t)$ is constructed using pilot simulations from model itself (we explore a similar idea in Section \ref{sec:quadrature} where we use quadrature integration instead of importance sampling).  More recently, \citet{guarniero2017iterated} introduce the \emph{iterated auxiliary particle filter} (iAPF).  The iAPF builds on the APF by iteratively refining a parametric approximation of a recursive factorization of the full backwards message, $p_{\btheta}(\by_{t+1:T} \mid \bx_t)$, as a function of $\bx_t$.  This refinement reuses forward simulations from the (iA)PF on the previous step.  This iterative procedure converges to a low-variance evidence estimate and set of posterior samples for a particular dataset.  \citet{heng2020controlled} builds on this general theme with \emph{controlled sequential Monte Carlo} (cSMC).  Instead of re-fitting the twisting potentials to the whole corpora of particles at each iteration, it cSMC instead fits an additional twist at each iteration to the residual from the previous iteration using approximate dynamic programming.  As such, they can provide a concrete estimate of the improvement per iteration.  

\todo{Needs very careful wording.}However, the methods we present are different in a number of crucial ways to \citet{guarniero2017iterated} and \citet{heng2020controlled}.  Foremost, we also consider learning the model and proposal (using FIVO) jointly with the backwards message.  This extends the definition of FIVO to include a backwards message, just how twisted SMC extends filtering SMC to use a backwards message.   In terms of learning the backwards message, we pose the message as a ratio of densities, and use techniques from density ratio estimation (DRE) to model the backwards message as a binary classification logit.  On a low level, we also employ a different, and more flexible, family of approximations of the backwards message that do not require positing an explicit parametric distributional family for the twist function.  Finally, we also consider amortized inference, where a parameterized function approximator that accepts the observations themselves as inputs, are learned, as opposed to using an iterative method to analyze a single dataset.  

It is also important to note that using a twisted SMC sampler dictates that a different proposal compared to filtering SMC.  The sequence of target distributions is now conditioned on the whole dataset, and hence for the proposal to match the posterior distribution (as is required to achieve a tight variational bound, see Section \ref{sec:methods:sixo_bound:tightness}), the proposal must also be conditioned on future information.  This also suggests that the bootstrap proposal may be inadequate for good performance in certain models.  Similarly, it is not sufficient to train a model and proposal using FIVO, and then fit a twist to the resulting lineages, without re-training the proposal.  \aw{this needs wording better.}

\subsection{Other Smoothing Approaches.}
\label{app:sec:background:other}
Our work is most similar in intent to \citet{kim2020variational}, who discuss using future likelihood estimates (twists) to create a lower-variance but still unbiased estimator of the IWAE gradient.  The backwards message is learned using temporal difference learning (similar to \citet{lawson2018twisted}).  It what shown by \citet{maddison2017filtering} that the FIVO bound is a tighter bound than the IWAE bound.  We show later that the SIXO bound is tighter still, and actually becomes tight at the optimal proposal (c.f. Section \ref{sec:background:fivo:sharpness}).  Therefore, our work can also be considered as transferring the same principle as \citet{kim2020variational} to sequential Monte Carlo, FIVO, and the tightness of the variational bound achieved.  \citet{kim2020variational} also reference the fact that the FIVO gradients that are used in practice are biased, whereas their IWAE bound is not biased.  In  a simple experiment in Section \ref{sec:exp:gdd}, we show that SIXO can recover a tight bound gap and optimal parameters even with biased gradients.  This provides evidence that explicitly twisting the filtering targets to the smoothing targets helds to reduce the bias induced by dropping the high-variance gradient terms.  However, theoretical proof of this claim is defered to future work. \todo{not sure if this final point holds if biased fivo also recovers the correct parameters.}

\citet{park2020inference} consider learning a parametric look-ahead twist conditioned on a finite window of future data.  The length of this window can be considered as interpolating between filtering and smoothing, tending towards fully smoothing for longer windows.  We discuss windowed twists in Section \ref{sec:methods:learning:window}, but ultimately find them to be disadvantageous compared to the methods we present in Section \ref{sec:methods:learning:bwd}, as they have complexity per particle that is linear in the length of the window.  As a result, evaluating the twist may be significantly more computationally expensive that of iterating the model.  Furthermore, \citet{park2020inference} do not discuss model learning.  

\citet{moretti2020variational} consider generating smoothing distributions by using the a forwards-filtering backwards smoothing approach.  This bidirectional approach allows a particle to be assigned as an ancestor to a later particle.  This ``rewiring'' of particle lineages can reduce variance.  However, it still suffers the same intrinsic flaw as filtering SMC, in that regions of state space that are low-probability under the filtering distribution, but that are high probability under the smoothing distribution, may be under-sampled in a forward filtering pass, resulting in few particles dominating in the backwards pass.  For

\todo{AW->DL:  this is the squiffy paper you reviewed.  I agree that they just add future obs to the proposal and that is wrong.  Its also only a workshop paper.  I think we might just leave it out, as opposed to trying to tear them down here.}  Finally, \citet{moretti2019smoothing} consider smoothing within the FIVO framework.  However, to achieve smoothing, they tie the forward weights of a learned proposal to that of the generative model.  \todo{finish.}
